# Supplementary material for: Regularity Conditions for Critical Point Convergence
Source: arXiv:2507.01854 source file (2025-08-08)
Supplement: Supplementary file 1 [file Supplementary.pdf]

# Regularity Conditions for Critical Point Convergence

## Supplementary Material

Thomas J. Maullin-Sapey<sup>1</sup> and Samuel Davenport<sup>2</sup>

<sup>1</sup>School of Mathematics, University of Bristol, Bristol, United Kingdom

<sup>2</sup>Division of Biostatistics, University of California, San Diego, CA, USA

## 1 Empirical Processes Background Material

In this supplement, we give background definitions and additional lemmas for the empirical processes theory employed in Section ?? of the main document. The framework we employ is based on that of [1], which serves as a canonical reference for much of the below. To begin, we define the notions of *inner* and *outer* probability.

**Definition 1** (Inner and Outer Probability). Let  $(\Omega, \mathcal{F}, \mathbb{P})$  be a probability space. The *outer* and *inner probability*,  $\mathbb{P}^*$  and  $\mathbb{P}_*$  are defined as follows: for  $B \subseteq \Omega$ ,

$$\mathbb{P}^*[B] = \inf\{\mathbb{P}[A] : A \supseteq B, A \in \mathcal{F}\},$$

$$\mathbb{P}_*[B] = 1 - \mathbb{P}^*[\Omega \setminus B],$$

respectively.

Next, we define the convergence notions used in the main text as follows:

**Definition 2** (Convergence Notions for Empirical Processes). Let  $\{X_n\}_{n \in \mathbb{N}}$  and  $X$  be random processes on the probability space  $(\Omega, \mathcal{F}, \mathbb{P})$ . We say that:

- $X_n$  converges weakly to  $X$ , denoted  $X_n \rightsquigarrow X$ , if:

$$\lim_{n \rightarrow \infty} \mathbb{P}^*[X_n \in B] = \lim_{n \rightarrow \infty} \mathbb{P}_*[X_n \in B] = \mathbb{P}[X \in B],$$

for all Borel sets  $B$  such that  $\mathbb{P}[X \in \partial B] = 0$ .

- $X_n$  converges in outer probability to  $X$ , denoted  $X_n \xrightarrow{P^*} X$ , if:

$$\forall \epsilon > 0, \quad \lim_{n \rightarrow \infty} \mathbb{P}^*[|X_n - X| > \epsilon] = 0,$$

- $X_n$  converges almost uniformly to  $X$ , denoted  $X_n \xrightarrow{a.u.} X$ , if:

$\forall \epsilon > 0, \exists$  measurable  $A$  such that  $\mathbb{P}[A] \geq 1 - \epsilon$  and  $|X_n - X| \rightarrow 0$  uniformly on  $A$ .

*Remark.* For further detail see Theorem 1.3.4 and Definition 1.9.1 of [1].

Also appearing in the statement of Theorems ?? and ?? of the main text is the notion of separability, defined as follows:

**Definition 3** (Separable Random Variable). An arbitrary set  $A$  is said to be separable if it contains a countable dense subset. A random variable  $X$  is said to be separable if there exists a separable measurable set,  $V$ , such that  $\mathbb{P}[X \in V] = 1$ .

Below is the variant of the Borel-Cantelli Lemma used in the proofs of Theorems ?? and ?? of the main text. Although a standard result of probability theory, the version we employ uses the outer probability measure, which may be unfamiliar to some, hence it's inclusion below.

**Lemma 1** (Borel-Cantelli). *Let  $E_1, E_2, \dots$  be a sequence of events  $(\Omega, \mathcal{F}, \mathbb{P})$ . Then, the below implication holds:*

$$\sum_{n=1}^{\infty} \mathbb{P}^*(E_n) < \infty \quad \implies \quad \mathbb{P}^* \left[ \limsup_{n \rightarrow \infty} E_n \right] = 0.$$

*Proof.* The proof for the outer measure case is identical to the standard proof of Borel-Cantelli, c.f. Chapter 1 of [2].  $\square$

Also employed is the below version of almost sure representation theorem for empirical processes and the subsequent lemma relating convergence in outer probability and weak convergence.

**Theorem 1** (Almost Sure Representations). *Let  $\{X_n\}_{n \in \mathbb{N}}, X : \Omega \rightarrow \mathbb{D}$  be random processes on the probability space  $(\Omega, \mathcal{F}, \mathbb{P})$ , where  $\mathbb{D}$  is a metric space. If  $X_n \rightsquigarrow X$  and  $X$  is separable, then there exist measurable maps  $\tilde{X}_n : \tilde{\Omega} \mapsto \mathbb{D}$  defined on some probability space  $(\tilde{\Omega}, \tilde{\mathcal{F}}, \tilde{\mathbb{P}})$  with:*

- (i)  $\tilde{X}_n \xrightarrow{a.u.} \tilde{X}$ ,
- (ii)  $\tilde{X}_n$  and  $X_n$  are equal in law on  $\mathbb{D}$  for all  $n$ .

*Proof.* See Theorem 1.10.3 of [1].  $\square$

**Lemma 2** (Convergence in Outer Probability Implies Weak Convergence). *Let  $\{X_n\}_{n \in \mathbb{N}}$  and  $X$  be random variables on the probability space  $(\Omega, \mathcal{F}, \mathbb{P})$ , where  $X$  is Borel measurable. If  $X_n \xrightarrow{P^*} X$  then  $X_n \rightsquigarrow X$ .*

*Proof.* See Lemma 1.10.2 (ii) of [1].  $\square$

## 2 Manifolds

As the definitions often vary between sources, in this supplement, we provide an explicit definition of the terms ‘topological manifold’ and ‘smooth structure’. For further detail, we recommend [3]. A topological manifold is defined as follows:

**Definition 4** (Topological Manifold). A topological space  $S$  is said to be a  $D$ -dimensional manifold or  $D$ -manifold, if it satisfies the following properties:

- $S$  is *Hausdorff*: for all distinct  $p, q \in S$ , there exist disjoint open sets  $U, V \subset S$  with  $p \in U$  and  $q \in V$ .
- $S$  is *second countable*: the topology of  $S$  has a countable basis.
- $S$  is *locally Euclidean of dimension  $D$* : every point of  $S$  has a neighbourhood which is homeomorphic to an open ball in  $\mathbb{R}^D$ .

If  $\mathbb{R}^D$  is replaced with  $\mathbb{H}^D$  in the last bullet point, where  $\mathbb{H}^D := \{(x_1, \dots, x_D) \in \mathbb{R}^D : x_D \geq 0\}$  is the  $D$ -dimensional upper half plane, we say that  $S$  is a  $D$ -manifold with boundary.

As we always denote the dimension as  $D$ , we use ‘ $D$ -manifold’ and ‘manifold’ interchangeably. It is worth noting that, as every open subset of  $\mathbb{R}^D$  can be seen to be homeomorphic to an open subset of  $\mathbb{H}^D$ , we have that every manifold is a manifold with boundary, but the converse is not true.

We next define what is meant by a  $C^k$  map (alternatively, a  $C^k$  function) on  $\mathbb{R}^D$ . Given an open subset  $U \subset \mathbb{R}^D$ , we say that a function  $f : U \rightarrow \mathbb{R}$  is  $C^k$  if it has partial derivatives of order less than or equal to  $p$  which are continuous over  $U$ . For an arbitrary subset  $V \subset \mathbb{R}^D$ , we say  $g : V \rightarrow \mathbb{R}$  is  $C^k$  if every point of  $V$  has a neighborhood over which  $g$  extends to a  $C^k$  function. If a  $C^k$  map has a  $C^k$  inverse, we say that it is a  $C^k$ -diffeomorphism.

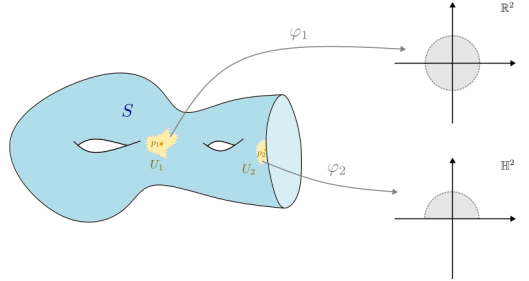

Figure 1: Two charts,  $(U_1, \varphi_1)$  and  $(U_2, \varphi_2)$ , on a manifold with boundary  $S$ .

Given a topological manifold  $S$ , we say that  $(U, \varphi)$  is a *chart* for  $S$  if  $U \subset S$  is open and the *coordinate map*  $\varphi$  is a homeomorphism from  $U$  to an open subset of  $\mathbb{R}^D$ . In this case,  $U$  is known as the domain of the chart. A collection of charts whose domains cover  $S$  is an *atlas* for  $S$ . A  $C^k$  *atlas* is an atlas which satisfies the following condition: if  $(U, \varphi)$  and  $(V, \psi)$  are charts in the atlas, then either  $U \cap V = \emptyset$  or  $(\psi \circ \varphi^{-1}) : \varphi(U \cap V) \rightarrow \psi(U \cap V)$  is a  $C^k$  diffeomorphism. A  $C^k$  atlas is said to be a  $C^k$  structure on  $S$  if there is no larger  $C^k$  atlas which properly contains it. This definition can be generalized to manifolds with boundary by replacing  $\mathbb{R}^D$  with  $\mathbb{H}^D$  in the first sentence of this paragraph.

**Definition 5** ( $C^k$  Manifold with Boundary). A  $C^k$  manifold with boundary is a pair  $(S, \mathcal{A})$  where  $S$  is a topological manifold with boundary and  $\mathcal{A}$  is a  $C^k$  structure on  $S$ . When the  $C^k$  structure  $\mathcal{A}$  is understood, it is often omitted from the notation and we simply say that  $S$  is a  $C^k$  manifold with boundary.

*Remark.* An analogous definition holds for  $C^k$  manifolds (without boundary).

A function  $f : S \rightarrow \mathbb{R}$  is said to be a  $C^k$  function on  $S$  if  $f \circ \varphi^{-1}$  is a  $C^k$  function on  $\mathbb{R}^D$  for each coordinate chart  $(U, \varphi)$  in a smooth structure on  $S$ .

### 3 Singular Homology

In this supplement, we provide a brief overview of singular homology, making explicit the notation used in the main document. Many of the conventions we adopt follow those of [3] Chapters 5, 9 and 13, to which we refer the reader for further detail. To begin we define the *standard  $p$ -simplex*, which broadly speaking is a  $p$ -dimensional triangle in  $\mathbb{R}^D$ .

**Definition 6** (Standard  $p$ -simplex). A  $p$ -dimensional simplex is a set of the form:

$$[v_1, \dots, v_p] := \left\{ x_1 v_1 + \dots + x_p v_p : \sum_{i=1}^p x_i \leq 1 \text{ and } x_i \in \mathbb{R}_{\geq 0} \text{ for all } i. \right\}$$

The standard  $p$ -simplex  $\Delta_p \subseteq \mathbb{R}^{p+1}$  is defined as  $\Delta_p = [e_0, \dots, e_p]$  where  $e_0$  is the  $p$ -dimensional zero vector and  $e_i = (0, \dots, 1, \dots, 0)$  is the  $i^{\text{th}}$  standard unit vector in  $\mathbb{R}^{p+1}$  with the  $i^{\text{th}}$  element equal to 1 and all other elements equal to 0.

To generalize the notion of simplex from  $\mathbb{R}^D$  to an arbitrary manifold with boundary,  $S$ , we define the ‘singular  $p$ -simplex’, which describes how a standard  $p$ -simplex is mapped into  $S$ . The name singular originates from the fact that the mapping may be degenerate (meaning, for example, a singular  $p$ -simplex may map a 2-dimensional triangle in  $\mathbb{R}^3$  to a one dimensional line in  $S$ ).

**Definition 7** (Singular  $p$ -simplex). A singular  $p$ -simplex is a continuous map  $\sigma : \Delta_p \rightarrow S$ .

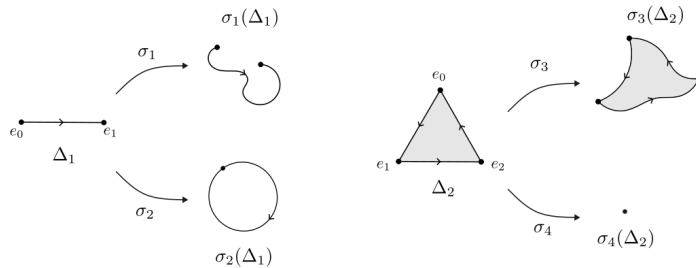

Figure 2: Two examples of singular 1-simplices,  $\sigma_1, \sigma_2 : \Delta_1 \rightarrow \mathbb{R}^2$ , and two examples of singular 2-simplices,  $\sigma_3, \sigma_4 : \Delta_2 \rightarrow \mathbb{R}^2$ .

We next define the free Abelian group on an arbitrary set  $X$ . In words, this group treats the elements of  $X$  as though they can be, in some sense, multiplied by integers and summed together. The group then consists of all “*formal linear combinations*” of the elements of  $X$ , under the presumed addition operation.

**Definition 8** (Free Abelian group). The free Abelian group on a non-empty set  $X$  is the set of formal linear combinations of  $X$ :

$$\mathbb{Z}X = \left\{ \sum_{i=1}^m n_i x_i : m \in \mathbb{Z}, \text{ for all } i, x_i \in X, n_i \in \mathbb{Z} \right\}$$

Given this definition, we can now define ‘*chains*’ of simplices, which are simply collections of singular simplices of a given dimension. This name is inspired by the fact that we may wish to ‘chain together’ a sequence of singular 1-simplices (one-dimensional lines) to obtain a longer 1-simplex, or a more complex combination of 1-simplices such as a loop or graph. The idea extends naturally to higher dimensions, but is harder to visualize.

**Definition 9** (Singular Chain Group). The *singular chain group of dimension  $p$* ,  $C_p(S)$ , is the free Abelian group on the set of all singular  $p$ -simplices. The elements of  $C_p(S)$  are formal linear combinations of singular  $p$ -simplices, referred to as singular  $p$ -chains or, as used throughout this work, simply as  $p$ -chains.

Next we define the ‘*faces*’ of a singular  $p$ -simplex. As a singular  $p$ -simplex is a map from a standard simplex to  $S$ , we also define the face of a singular  $p$ -simplex as a map; this time, one which maps the standard  $(p-1)$ -simplex to a single face of the standard  $p$ -simplex (see Fig. 3).

**Definition 10** (Face Map). The  $i^{\text{th}}$  face map in dimension  $p$ ,  $F_{i,p} : \Delta_{p-1} \rightarrow \Delta_p$ , is defined by the unique affine mapping  $[e_0, \dots, e_{p-1}] \mapsto [e_0, \dots, e_{i-1}, e_{i+1}, \dots, e_p]$ .

This definition is useful as it allows us to characterize the relation between singular simplices of different dimensions. Specifically, it allows us to define the boundary operator, which maps a  $p$ -simplex to a signed combination of its  $(p-1)$ -dimensional faces.

**Definition 11** (Boundary operator). The  $p$ -dimensional boundary operator,  $\partial : C_p(S) \rightarrow C_{p-1}(S)$  (sometimes denoted  $\partial_p$ ) is the unique group homomorphism satisfying:

$$\partial\sigma = \sum_{i=0}^p (-1)^i \sigma \circ F_{i,p},$$

for any arbitrary singular  $p$ -simplex  $\sigma$ .

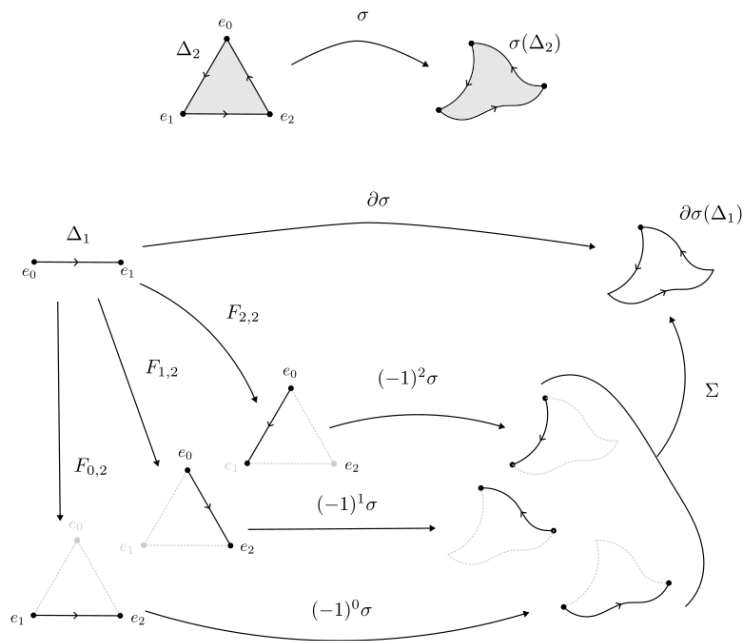

Figure 3: Illustration of the boundary operator and face map.

The notion of the boundary operator is extremely powerful, as it allows us to define the notions of cycles and boundaries for arbitrary singular simplices.

**Definition 12** (Cycles and Boundaries). A  $p$ -cycle is a  $p$ -chain  $c$  satisfying  $\partial c = 0$  and a  $p$ -boundary is a  $p$ -chain  $c$  satisfying  $\partial b = c$  for some  $b \in C_{p+1}(S)$ . The subgroup of  $C_p(S)$  of  $p$ -cycles on  $S$  is denoted  $Z_p(S) := \text{Ker}(\partial_p)$  and the subgroup of  $C_p(S)$  of  $p$ -boundaries on  $S$  is denoted  $B_p(S) := \text{Im}(\partial_{p+1})$ .

We are now in a position to define the singular homology groups which consist of the ‘unique cycles’ in a space which are not boundaries. Informally, the  $p^{th}$  homology group can be thought of as the group generated by the “unique holes” of dimension  $p$  in a space. For instance, the 1-dimensional homology group of  $\mathbb{S}$  is the group  $\{m[l] : m \in \mathbb{Z}\}$  where  $[l]$  represents the loop starting at 1 and traversing the circle clockwise once, and  $m[l]$  represents the path obtained by traversing this loop  $m$  times.

**Definition 13** ( $p^{th}$  Singular Homology Group). The  $p^{th}$  singular homology group is the quotient group:

$$H_p(S) := Z_p(S)/B_p(S) = \text{Ker}(\partial_p)/\text{Im}(\partial_{p+1}) \quad (1)$$

The equivalence class of the  $p$ -cycle  $c \in Z_p(S)$  in  $H_p(S)$  is denoted by  $[c]$  and referred to as its '*homology class*'.

A standard result of homology theory, extending the previous example is the following:

**Lemma 3.** For any  $n \in \mathbb{N}$ ,  $H_n(\mathbb{S}^n) \cong \mathbb{Z}$ . That is,  $H_n(\mathbb{S}^n)$  is an infinite cyclic group generated by a single element.

*Proof.* See [3] Theorem 13.23 (Homology Groups of Spheres).  $\square$

A map from a space  $S$  to a space  $T$  can be converted to a corresponding map between classes of cycles in  $H_p(S)$  and classes of cycles in  $H_p(T)$  as follows.

**Definition 14** (Induced Homomorphism). If  $f : S \rightarrow T$  is a continuous map, it is said to induce a (group) homomorphism  $f_{\#} : C_p(S) \rightarrow C_p(T)$  defined by  $f_{\#}(\sigma) := f \circ \sigma$ . This homomorphism in turn passes to the quotient to induce another homomorphism  $f_* : H_p(S) \rightarrow H_p(T)$  satisfying  $f_* \circ q = f_{\#}$ , where  $q$  is the quotient map associated with (1).

Given this last definition, it can be seen that if  $f : \mathbb{S}^q \rightarrow \mathbb{S}^q$  is a continuous map, it must induce a group homomorphism  $f_* : H_q(\mathbb{S}^q) \rightarrow H_q(\mathbb{S}^q)$ . Given Lemma 3, we can think of  $f_*$  as an homomorphism from  $\mathbb{Z}$  into  $\mathbb{Z}$ , from which it follows that  $f_*$  can be represented uniquely by a mapping of the form  $z \mapsto \alpha \cdot z$  for some  $\alpha \in \mathbb{Z}$ . We now define the degree of a map  $\varphi : \mathbb{S}^q \rightarrow \mathbb{S}^q$  as follows:

**Definition 15** (Degree of a Map on Spheres). Let  $\varphi : \mathbb{S}^q \rightarrow \mathbb{S}^q$  be a continuous map. The degree of  $\varphi$ ,  $\deg(\varphi)$ , is defined as the unique integer  $\alpha$  satisfying:

$$\varphi_*([c]) = \alpha \cdot [c],$$

where  $\varphi_*$  is the induced homomorphism from  $H_q(\mathbb{S}^q)$  to  $H_q(\mathbb{S}^q)$  and  $[c]$  is an arbitrary homology-class in  $H_q(\mathbb{S}^q)$ .

In words, the degree describes how many times the map  $\varphi$  maps  $\mathbb{S}^q$  onto itself. For instance, if  $\varphi : \mathbb{S}^1 \rightarrow \mathbb{S}^1$  is defined by  $\varphi(e^{i\theta}) = e^{\alpha i\theta}$ ,  $\alpha \in \mathbb{Z}$ , induces the homomorphism  $\varphi_* : H_1(\mathbb{S}^1) \rightarrow H_1(\mathbb{S}^1)$  which maps  $[c] \mapsto \alpha[c]$ . Here,  $\varphi$  takes the circle  $\mathbb{S}^1$  and ‘wraps it around itself’  $\alpha$  times (see Fig. 4). This notion of degree is used in Definition ?? of the main text.

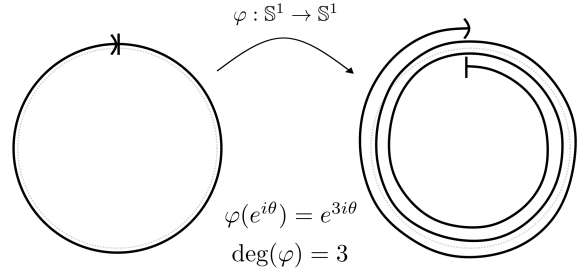

Figure 4: Illustration of the topological degree.

## 4 Orientability

In this section, we make explicit what is meant by *orientability* of a manifold. Much of the notation is drawn from that of [4] Sections 2.1 and 3.3, to which we refer the reader for further detail. To define what we mean by orientable, we now define the relative homology group of  $A$  in  $X$ , which broadly speaking identifies chains in  $C_p(X)$  with chains in  $C_p(A)$ .

**Definition 16** ( $p^{th}$  Relative Singular Homology Group). Given a topological space  $S$  and a subspace  $T \subseteq S$ , we denote the quotient group  $C_p(S)/C_p(T)$  by  $C_p(S, T)$ . By passing  $\partial_p : C_p(S) \rightarrow C_{p-1}(S)$  to the quotient, in a slight abuse of notation, we define a new boundary operator  $\partial_p : C_p(S, T) \rightarrow C_{p-1}(S, T)$ . As in Equation (1), we then define the  $p^{th}$  relative singular homology group as:

$$H_p(S, T) := \text{Ker}(\partial_p) / \text{Im}(\partial_{p+1}).$$

By convention, we define  $H_p(S|T) := H_p(S, S \setminus T)$ . In the case that  $A = \{s\}$  for some  $s \in S$ , we write  $H_p(S|s) := H_p(S|\{s\})$ .

We are now able to define the local orientation of a space  $S$  at point  $s \in S$  as follows:

**Definition 17** (Local Orientation). A local orientation of a  $D$ -dimensional topological manifold  $S$  at point  $x$  is a choice of generator  $\mu_s$  for the infinite cyclic group  $H_D(S|s)$ .

In words, a local orientation can be thought of as a generalization of the notion of ‘clockwise’ and ‘anticlockwise’ to arbitrary dimensions. For instance, a local orientation for  $\mathbb{R}^2$  at  $s \in \mathbb{R}^2$  is a choice of generator for the infinite cyclic group  $H_2(\mathbb{R}^2|\{s\}) \cong H_1(\mathbb{S}^1)$  (c.f. [4] Section 3.3 ‘Orientations and Homology’). The only choices for a generator of  $H_1(\mathbb{S}^1)$  are the loop tracing the circle clockwise, and the loop tracing the circle counterclockwise. Therefore, specifying a local orientation for  $H_2(\mathbb{R}^2|\{s\})$  is the same as deciding whether to treat loops around  $\{s\}$  as being either clockwise or anti-clockwise ‘by default’.

In order to define a ‘global orientation’ for a manifold  $S$ , we need to place some form of condition on the local orientations to ensure that points close to one another are ‘similarly oriented’. This is achieved by the below definition:

**Definition 18** (Global Orientation). The mapping  $s \rightarrow \mu_s$  is a *global orientation* for  $S$  if every  $s \in S$  has a neighborhood  $U$  such that the local orientations for all  $s' \in U$  are the image of a single generator of  $H_D(S|U)$ . If an element  $[c]$  of  $H_D(S)$  is a generator of  $H_D(S|s)$  for all  $s$ , then we say that  $[c]$  is a *fundamental class* of  $S$ .

The condition in the above definition is often described as a ‘local consistency’ condition, as it ensures that points which are close to one another have orientations that are in some sense ‘consistent’ with one another. Given the above definitions, a natural question is when a topological manifold  $S$  has a fundamental class. This is answered by the below theorem:

**Theorem 2.** *If  $S$  is a compact, connected, orientable  $D$ -dimensional manifold, then  $S$  has a fundamental class  $[c] \in H_D(S)$ .*

*Proof.* See Theorem 3.26 (a) of [4]. Note this proof uses a generalized notion of orientability,  $R$ -orientability, which we have not used for brevity.  $\square$

## 5 Construction of the Surfaces in Figure ??

In this section, we provide the equations used to construct the surfaces shown in Figure ?? of the main document. For the surface in (a), we begin by defining the smooth bump function,  $b : \mathbb{R} \rightarrow \mathbb{R}$ , and smooth transition function  $T : \mathbb{R} \rightarrow \mathbb{R}$  by:

$$b(x) := \begin{cases} e^{-\frac{1}{1-x^2}} & \text{if } |x| < 1, \\ 0 & \text{otherwise,} \end{cases} \quad \text{and} \quad T(x) := \begin{cases} 0 & \text{if } x \leq 0, \\ \frac{x^2}{x^2+(1-x)^2} & \text{if } 0 < x < 1, \\ 1 & \text{otherwise.} \end{cases}$$

Following this, we define the semi-circle function  $s(x) := \sqrt{1-x^2}$  if  $|x| < 1$  and 0 otherwise and let  $g : \mathbb{R} \rightarrow \mathbb{R}$  be the function:

$$g(x) := x + T(4x-1)(s(x)-x) + T(4x-3)(x-s(x))$$

In words, the graph of  $g$  appears to look like  $y = x$  for  $x \notin (1/4, 1)$  but smoothly transitions into a circular arc for  $x \in (1/2, 3/4)$ . The graph of  $g$  is exactly the contour line shown on the bottom left of Fig. ?. To construct the surface shown in ?? (a), we then define  $f$  as follows:

$$f(x, y) = c + y - g(x) + b(5\sqrt{x^2 + y^2})(x - y - x^3 + y^3)$$

Ignoring the constant  $c$ , the first term,  $y - g(x)$ , extends the graph of  $g$  out in three dimensions to form a slope. As  $g(x) = x$  near the origin,  $y - g(x) = y - x$  on a suitably small region. To ensure  $f$  has a critical point at the origin, the bump function term then deforms a small neighborhood of the origin to look like  $x^3 - y^3$ . This has the effect of inducing a point of undulation at the origin.

For (b), we begin by defining the function  $h : \mathbb{R} \rightarrow \mathbb{R}$  by:

$$h(x) = x^2 \sqrt{\sin(10/x)} \frac{\sin(10/x)}{|\sin(10/x)|}.$$

Visually,  $h$  looks like the graph of  $x^2 \sin(1/x)$ , but adjusted to have infinite gradient whenever  $h$  crosses the axis. The graph of  $h$  is exactly the contour shown in the bottom right of Fig. ?? (b). The surface shown in (b) is now given by  $f(x, y) := c + x(y - h(x))$ , which can be trivially seen to have non-zero gradient for all  $(x, y) \neq (0, 0)$  but possess a saddle at the origin. As the graph of  $h$  has infinite gradient whenever it crosses the  $x$ -axis, it follows that  $\nabla f$  is normal to  $f^{-1}(c)$  whenever  $f^{-1}(c)$  crosses the line  $x = 0$ . Thus the set  $\mathcal{K}$  consists of points where  $f^{-1}(c)$  crosses  $x = 0$ , as illustrated.

## 6 The Cantor-Thirds Counterexample

In Section ?? of the main text, we noted that much of our working could have been simplified if we were permitted to assume the following: for any  $f \in C^1(S, \mathbb{R})$  with a single isolated critical point  $p$  satisfying  $f(p) = c$ , there exists a  $\delta > 0$  such that  $\partial B_\delta(p)$  intersects the level set  $f^{-1}(c)$  transversally. However, as we discussed there, it is possible to construct a function  $f \in C^1(S, \mathbb{R})$  for which this condition fails. In the main text, the existence of such an example necessitated the introduction of Lemma ?. In what follows, we justify the need for this lemma by providing an explicit construction of such a function.

To be specific, in this section we outline the construction of a  $C^1$  function  $f : B_1 \rightarrow \mathbb{R}$ , where  $B_1 \subset \mathbb{R}^3$  is the open unit ball centered at the origin. This function has a single isolated critical point at the origin, with  $f(0) = 0$ , and possesses the unusual property that the level set  $f^{-1}(0)$  intersects  $B_\delta$  tangentially for every  $\delta \in (0, 1)$ . We refer to this as the *Cantor-thirds counterexample*, due to its reliance on well-known properties of the Cantor Ternary set. Here, we provide only the broad strokes of the construction; further details, along with explicit expressions and code for generating the accompanying figures, can be found at the following repository:

<https://www.github.com/TomMaullin/Cantor-Counter>

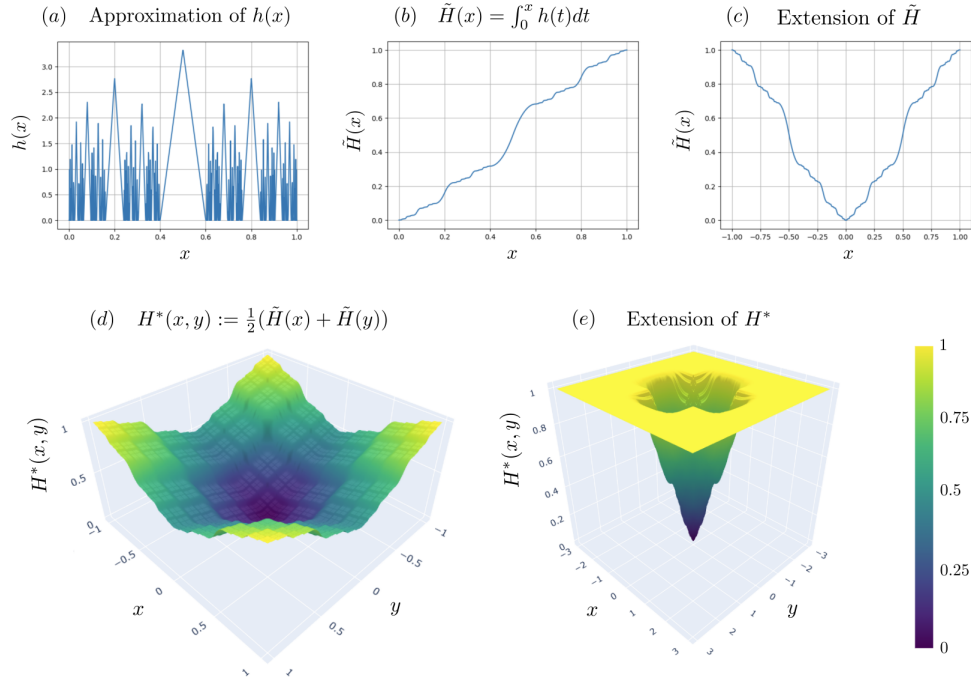

Figure 5: Construction of the function  $H^*$ . (a) The function  $h : [0, 1] \rightarrow \mathbb{R}$  is constructed by summing carefully positioned ‘spikes’ of decreasing height and width. (b)  $h$  is defined such that  $\tilde{H}(x) := \int_0^x h(t) dt$  has a critical point at every level  $c$  in the Cantor ternary set. (c) The definition of  $\tilde{H}$  is extended to be symmetric about the origin. (d) The function  $H^* : [-1, 1]^2 \rightarrow [0, 1]$  is defined as  $H^*(x, y) := \frac{1}{2}(\tilde{H}(x) + \tilde{H}(y))$ . For every  $z \in [0, 1]$ , there exists a point  $(x, y) \in [-1, 1]^2$  such that  $\nabla H^*(x, y) = 0$  and  $H^*(x, y) = z$ . (e)  $H^*$  is extended to all of  $\mathbb{R}^2$  using a  $C^1$  transition function, with  $H^*(x, y) = 1$  for all  $(x, y) \notin [-2, 2]^2$ .

## 6.1 Constructing $H^*$

We begin by constructing a  $C^1$  function  $H^* : \mathbb{R}^2 \rightarrow [0, 1]$  that has a critical point at every level  $z \in [0, 1]$ . More precisely,  $H^*$  satisfies the property that for every  $z \in [0, 1]$ , there exists a point  $(x, y) \in [0, 1]^2$  such that  $\nabla H^*(x, y) = 0$  and  $H^*(x, y) = z$ . To construct  $H^*$ , we first adopt the approach outlined by [5], which proceeds as follows.

We first define a function  $h : [0, 1] \rightarrow \mathbb{R}$  as an infinite sum of triangular “spikes” with decreasing height and width. These spikes are positioned so that the integral of  $h$ , denoted  $\tilde{H}(x) := \int_0^x h(t) dt$ , has a critical point at every level  $c \in C$ , where  $C \subset [0, 1]$  denotes the middle-thirds Cantor set. This is achieved by ensuring that the cumulative area under  $h$  matches exactly the distribution of values in  $C$ , exploiting its self-similar structure. Illustrations of  $h$  and  $\tilde{H}$  are provided in Fig. 5 (a) and (b), respectively. The function  $\tilde{H}$  is then extended to an even function on the interval  $[-1, 1]$ , preserving its differentiability at the origin (Fig. 5 (C)).

Next, a two-variable function  $H^* : [-1, 1]^2 \rightarrow [0, 1]$  is defined by combining the values of  $\tilde{H}$  along each coordinate axis:

$$H^*(x, y) := \frac{1}{2} \left( \tilde{H}(x) + \tilde{H}(y) \right).$$

This construction ensures that every level  $z \in [0, 1]$  contains a critical point of  $H^*$ , due to the additive property  $C + C = [0, 2]$  of the Cantor set. Illustration of  $H^*$  is provided in Fig. 5 (d).

Finally,  $H^*$  is extended to a function on all of  $\mathbb{R}^2$  by means of a  $C^1$  transition function, which interpolates between the above definition on  $[-1, 1]^2$  and the constant value 1 outside the larger square  $[-2, 2]^2$ . The resulting function remains globally  $C^1$ , with critical points densely distributed across all levels in the interval  $[0, 1]$  (see Fig. 5 (e)).

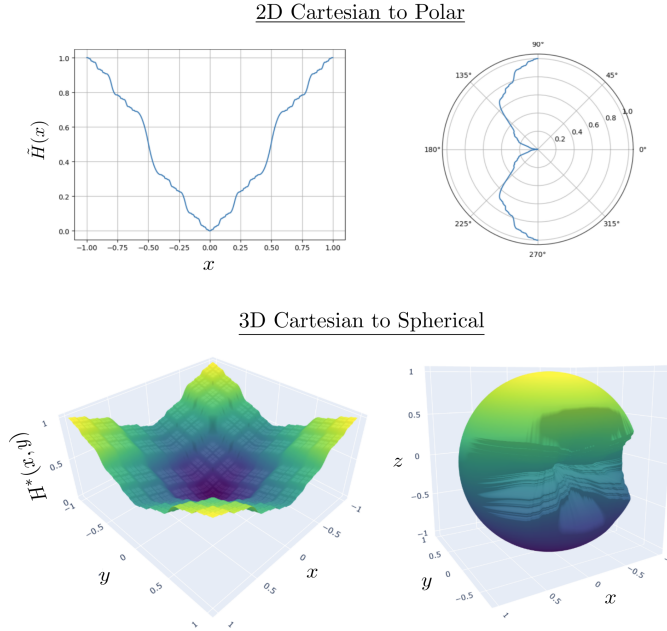

Figure 6: Top row: Transforming the graph  $y = \tilde{H}(x)$  (left) to the polar equivalent  $r = \tilde{H}(2(\theta/\pi - 1))$  (right). Note how each critical point of level  $\delta$  in the cartesian plot is mapped to a point tangent to  $B_\delta$  in the polar plot. Bottom row: The transformation from  $z = H^*(x, y)$  to  $r = H(\theta, \psi)$ . Again, critical points in the left plot are mapped to points which are tangential to the sphere on the right.

## 6.2 Mapping to the Sphere

Our aim is to now transform the surface described by  $z = H^*(x, y)$ , which tangentially intersects the plane  $z = \delta$  for all  $\delta \in [0, 1]$ , into a surface that is tangent to every ball  $B_\delta$  for  $\delta \in [0, 1]$ . Intuitively, this transformation can be thought of “wrapping” the original surface around a sphere’. To achieve this, we define a new function  $H : [0, \pi) \times [0, 2\pi) \rightarrow \mathbb{R}_{\geq 0}$  in spherical coordinates  $(\theta, \psi)$  by

$$H(\theta, \psi) := H^*\left(\frac{\pi}{2k}(\theta + k), \frac{\pi}{k}(\psi + k)\right)$$

for some suitably large integer  $k$ .

Geometrically, transforming the Cartesian graph  $z = H^*(x, y)$  to the spherical graph  $r = H(\theta, \psi)$  corresponds to embedding a plane containing the critical structure of  $H^*$ , onto the surface of a sphere of radius 1. If  $k$  is large, intuitively, one can think of this as removing a small ‘panel’ from the sphere and replacing it with a rescaled and slightly curved version of  $H^*$  that conforms to the spherical geometry. In our illustrations, including Fig. 6, we use a smaller value,  $k = 4$ , so that the embedded panel spans a larger portion of the sphere (roughly half), making the transformation easier to visualize.

Before considering a 3D illustration of  $H$ , it is informative to consider the 2D analogue of the transformation, which is shown in the top row of Fig. 6. There, the Cartesian graph  $y = \tilde{H}(x)$  is transformed into its polar equivalent  $r = \tilde{H}(2(\theta/\pi - 1))$ . Here, each critical point at level  $\delta$  in the Cartesian plot maps to a point tangent to the circle  $B_\delta$  in the polar plot. An analogous process occurs in three dimensions (Fig. 6, bottom row).

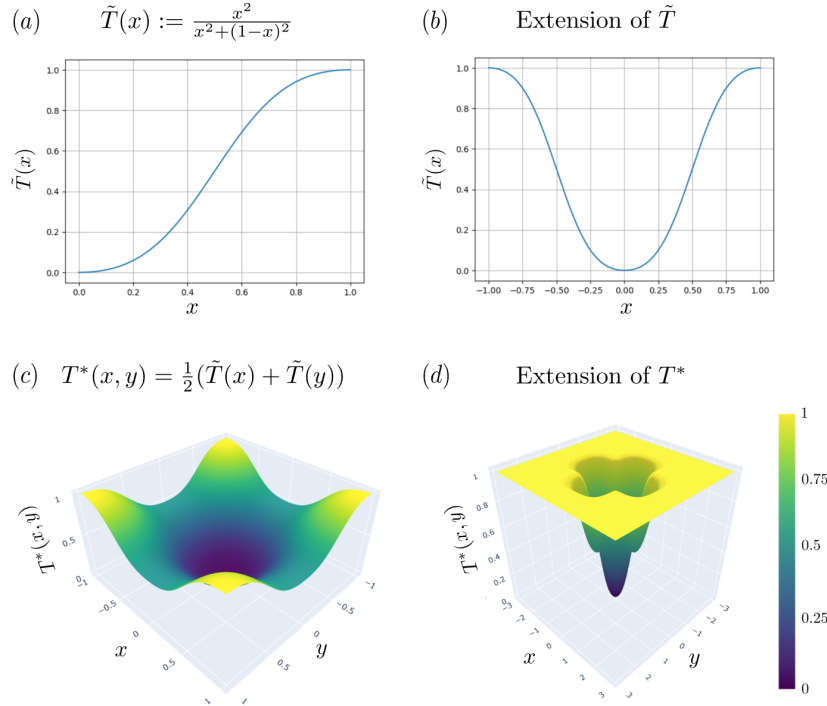

Figure 7: Construction of  $T^*$ . (a) As with the construction of  $H^*$ , we begin with a non-decreasing function  $\tilde{T}$  defined on  $[0, 1]$ . (b) We extend  $\tilde{T}$  to be even on  $[-1, 1]$ . (c)  $T^*$  is defined as a coordinate-wise average of  $\tilde{T}$ . (d)  $T^*$  is extended to  $\mathbb{R}^2$ , taking the constant value of 1 outside  $[-2, 2]^2$ .

### 6.3 Constructing $f$

We have now constructed a surface which is tangent to every sphere of radius  $\delta \in [0, 1]$ . To complete the counterexample, we must now construct a  $C^1$  function  $f : B_1 \rightarrow \mathbb{R}$  whose zero level set is the surface  $r = H(\theta, \psi)$  and whose only critical point is at the origin.

To this end, we must introduce a  $C^1$  transition function,  $\tilde{T} : [0, 1] \rightarrow [0, 1]$ , with positive gradient on  $(0, 1)$  and critical points at 0 and 1. One such function is  $\tilde{T}(x) = T(x)$  for  $x \in [0, 1]$ , where  $T$  is as defined in Supplementary Section 5. Using  $\tilde{T}$ , we then construct a  $C^1$  function  $T^* : \mathbb{R}^2 \rightarrow \mathbb{R}_{\geq 0}$  that equals  $\frac{1}{2}(\tilde{T}(x) + \tilde{T}(y))$  inside  $[0, 1]^2$  and is extended to be constant (equal to 1) outside  $[-2, 2]^2$ . The construction of  $T^*$  mirrors that of  $H^*$  and is illustrated in Fig. 7.

Next, we define  $f^* : \mathbb{R}^2 \times \mathbb{R}_{\geq 0} \rightarrow \mathbb{R}$  in cartesian coordinates as:

$$f^*(x, y, z) := -T^*(x, y)(z - H^*(x, y))z^2 - \mathbb{1}[z > H^*(x, y)](z - H^*(x, y))^2,$$

where  $\mathbb{1}[A]$  denotes the indicator function, which is 1 when condition  $A$  holds and 0 otherwise. Since  $f^*$  is composed of  $C^1$  functions, it is itself  $C^1$ . Moreover, it satisfies the following properties:

1. The zero level set of  $f^*$  is given by

$$(f^*)^{-1}(0) = \{(x, y, z) : z = H^*(x, y)\} \cup \{(x, y, z) : z = 0\}.$$

2. For all  $x, y \in \mathbb{R}$ , the gradient vanishes on the plane  $z = 0$ :  $\nabla f^*(x, y, 0) = 0$ .
3. For all  $x, y \in \mathbb{R}$  and  $z \in (0, \frac{1}{3})$ , the gradient  $\nabla f^*(x, y, z)$  is nonzero.

Full proofs of these properties are provided in the supplemental notebook. As  $f^*$  is difficult to visualize, Fig. 8 displays several slices of  $f^*$  of the form  $w = f^*(x, c, z)$  for fixed  $c \in [0, 2]$ .

We are now in a position to define the final function  $f : [0, \infty) \times [0, \pi] \times [0, 2\pi) \rightarrow \mathbb{R}$  in terms of spherical coordinates as:

$$f(r, \theta, \psi) := f^*\left(\frac{\pi}{2k}(\theta + k), \frac{\pi}{k}(\psi + k), 3r\right).$$

By construction, we have  $f(0, \theta, \psi) = 0$  for all  $\theta$  and  $\psi$ . Moreover, outside the region  $[\frac{\pi}{4}, \frac{3\pi}{4}] \times [\frac{\pi}{2}, \frac{3\pi}{2}]$  in angular coordinates, that is, for

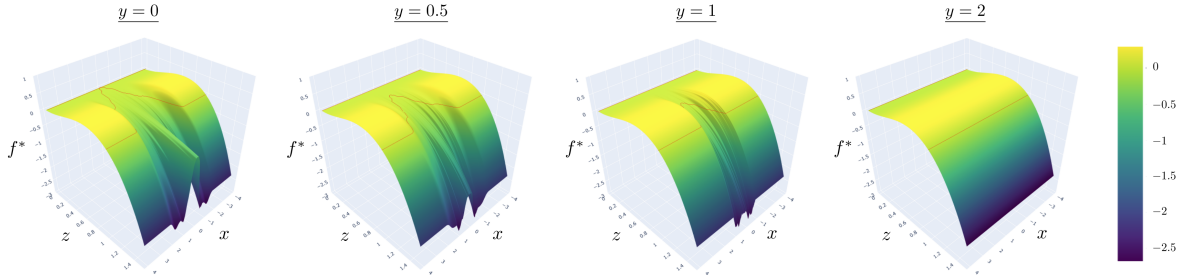

Figure 8: Slices of the function  $f^*(x, y, z)$  for  $y = 0, 0.5, 1$ , and  $2$ . Highlighted in red is the level set  $f^{-1}(0)$ , which consists of the union of the plane  $z = 0$  and the surface  $z = H^*(x, y)$  (cf. Fig. 5(e)). Since  $f^*$  is even in  $y$ , these slices are identical to those at  $y = -0.5, -1$ , and  $-2$ .

$$(r, \theta, \psi) \notin [0, \infty) \times \left[\frac{\pi}{4}, \frac{3\pi}{4}\right] \times \left[\frac{\pi}{2}, \frac{3\pi}{2}\right],$$

we have that

$$f(r, \theta, \psi) = -9(3r - 1)r^2 - \mathbb{1}[3r > 1](3r - 1)^2.$$

From this, it easily follows that  $f$  is a well defined function in terms of spherical coordinates. Further, by considering properties 2 and 3 of  $f^*$ , we see that  $f$  is  $C^1$  and has a single critical point at the origin. Finally, by Property 1 of  $f^*$ , and noting that the plane  $z = 0$  is mapped to the point  $r = 0$  under the transformation to spherical coordinates, it follows that the zero level set of  $f$  is exactly the desired spherical surface. Slices of  $f$ , viewed as a cartesian function, are visualized in Fig. 9.

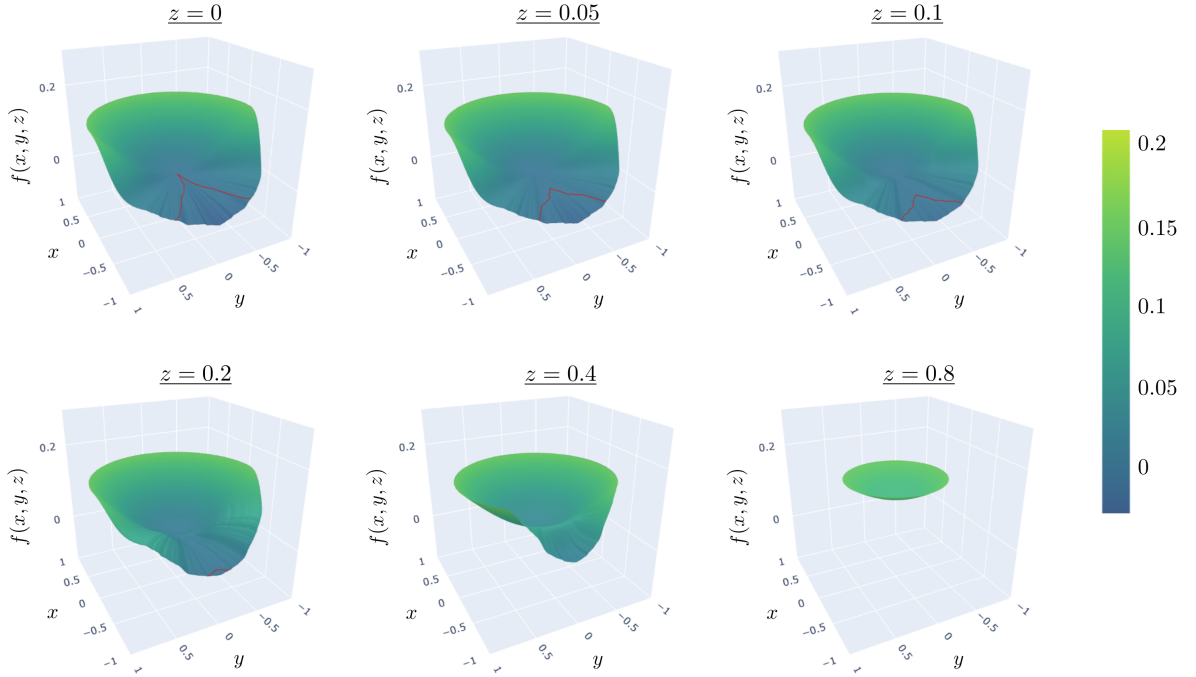

Figure 9: Slices of the function  $f(x, y, z)$  for fixed values  $z = 0, 0.05, 0.1, 0.2, 0.4$  and  $0.8$ . Highlighted in red is the level set  $f^{-1}(0)$ , which is a rescaled and cropped version of the spherical surface shown in the bottom right of Fig. 6. By construction,  $f$  has non-zero gradient everywhere except at the origin, and its zero level set tangentially intersects every ball of radius  $\delta \in [0, 1]$ .

## 7 Interactive Desmos Displays

Below is a list of interactive displays for the functions plotted in the main text, generated using the 2D and 3D Desmos graphics software packages:

- **Fig. ??:** <https://www.desmos.com/3d/zrraoa9ff2>
- **Fig. ??:** <https://www.desmos.com/3d/jfu5ayqk6p>

- **Fig. ??:** <https://www.desmos.com/3d/n6zfiejhpm>
- **Fig. ??(a):** <https://www.desmos.com/calculator/v6oaiv1e0h>
- **Fig. ??(b):** <https://www.desmos.com/calculator/zmeczgvgwwb>
- **Fig. ??(c):** <https://www.desmos.com/calculator/2hgkxtfmqb>
- **Fig. ??:** <https://www.desmos.com/3d/cj2uhtzozb>
- **Fig. ??:** <https://www.desmos.com/calculator/dwggzqkw2z>
- **Fig. ??:** <https://www.desmos.com/3d/nahl7yhbm3>
- **Fig. ??(a):** <https://www.desmos.com/calculator/hk6gtlkilg>
- **Fig. ??(b):** <https://www.desmos.com/3d/4fgjltaucr>
- **Fig. ??:** <https://www.desmos.com/3d/nlsl4fkfn2>
- **Fig. ??(a):** <https://www.desmos.com/3d/e6laacrpnh>
- **Fig. ??(b):** <https://www.desmos.com/3d/qgfkf1wau>
- **Fig. ??(a):** <https://www.desmos.com/calculator/6rqishj5fi>
- **Fig. ??(b):** <https://www.desmos.com/3d/3juuyn59qj>

## References

- [1] A. van der Vaart and J.A. Wellner. *Weak Convergence and Empirical Processes: With Applications to Statistics*. Springer Series in Statistics. Springer, 1996.
- [2] T. K. Chandra. *The Borel-Cantelli Lemma*. Springer Briefs in Statistics. Springer India, 2012.
- [3] J. Lee. *Introduction to Topological Manifolds*. Graduate Texts in Mathematics. Springer New York, 2010.
- [4] A. Hatcher. *Algebraic Topology*. Algebraic Topology. Cambridge University Press, 2002.
- [5] E. L. Grinberg. On the smoothness hypothesis in sard’s theorem. *The American Mathematical Monthly*, 92(10):733–734, 1985.
